# Supplementary material for: Towards a Problem-Oriented Domain Adaptation Framework for Machine Learning
Source: arXiv:2501.04528 source file (2025-01-08)
Supplement: Supplementary file 1 [file appendix.tex]

\section{Key Concepts}
\label{sec:concepts}

In the context of \ac{ML}, many concepts are firmly established and the average reader will likely be familiar with a majority if not all of the definitions in this chapter. In that case, \Ref{sec:appendix:concepts:tl} is still recommended as it explains important concepts for domain adaptation that might not be as present in other \ac{ML} contexts. Interested readers can follow along from the beginning for an introduction of concepts that starts at the basic definitions of \ac{ML} and successively moves towards the concepts relevant for domain adaptation.

\subsection{Machine Learning Foundations}
\label{sec:appendix:concepts:ml}
%Despite the firm establishment of machine learning as one of the disciplines of computer science, a common notation has not been fully established.  This section does not aim to propose a unified notation, but shall serve as an anchor point for the important concepts, the notation of which may be subject to change for different topics, authors, journals, etc. This is why in some cases, alternative notations are mentioned. Going further from the general idea of machine learning, a common notion is to define learning based on approximating an optimal hypothesis from a set of possible hypotheses so that a task is performed at the best possible performance. This leads to the definition of a learning machine as a hypothesis learner and subsequently of learning (in a narrow sense) as the estimation of a hypothesis. 

% \begin{definition}[Learning Machine]
% \label{LearningMachine}
% A learning machine uses learning methods to find the optimal hypothesis  \(h_{\alpha_{opt}}\) of given hypothesis space \(\{h_{\alpha}:\alpha \in A\}\) by looking at learning examples. The hypotheses are defined by parameters \(\alpha \in A\), whereas \(\alpha_{opt}\) are the parameters of the optimal hypothesis. A resulting decision or prediction model \(M_{opt}\) given by evaluating the optimal hypothesis.
%  \end{definition}
 
\begin{definition}[Learning.]
\label{Learning}
Learning is the estimation of a hypothesis \(h_{\alpha}(\vec{x})=y\) using (known) examples \((\vec{x}_1,y_1),...,(\vec{x}_n,y_n)\in X \times Y\) that are generated by a (unknown) system with probability \(P(\vec{x},y)\).
\end{definition}

A learning problem is defined by a set of attributes \(X\) and a set of correct outputs \(Y\). The correct output \(y\in Y\) is often referred to as the \emph{label} of a sample \(x \in X\). Typical learning problems are e.g., concept learning (\(y\in \{0,1\}\)), classification (\(y\in \{\text{class}_1,...,\text{class}_n\}\)), and regression (\(y \in \mathbb{R}\)). Choosing an optimal hypothesis requires a measure of quality, which is done by comparing the predictions of a hypothesis \(h_{\alpha}(\vec{x})\) for a given sample \(\vec{x}\) with the true label \(y\). This is called the error (of the model). 

\begin{definition}[Error.]
\label{def:Error}
A learning machine tries to estimate the hypothesis \(h\) so that it minimizes the error \(E(h)\):

\begin{equation}
E(h_{\alpha})=Func(h_{\alpha}(\vec{x}) \underset{\approx}{\leftrightarrow} y, P(\vec{x},y))
\end{equation}

whereas \(\underset{\approx}{\leftrightarrow}\) is a comparison between hypothesis output and target output. A great difference between hypothesis output and target output results in a high error. 
\end{definition}

This definition is not practical, because it does not specify how the difference between target and hypothesis output is calculated. For this end, a loss function must be defined. The precise calculation of the loss depends on the implementation. Common loss functions are e.g., binary, absolute error, or squared error.

\begin{definition}[Loss Function.]
\label{LossFunction}
Given a hypothesis \(h:X\rightarrow Y^{'}\), the loss function \(\ell\) is defined as 

\begin{equation}
\ell:(Y^{'}\times Y)\rightarrow \mathbb{R}
\end{equation}

and compares a sample's  prediction with its true label, or in some cases, with another learning machine's prediction. 
\end{definition}

Another practical challenge that is brought up by \Cref{def:Error}, is that often the real system \(P(\vec{x},y)\) is unknown, which means that a precise determination of this measure is not possible. Utilizing the loss function definition, a differentiation between a real and empirical error can be made based on what samples are used in the loss calculation.

\begin{definition}[Real Error.]
\label{RealError}
The real error is the error calculated via a given loss function \(\ell\) over all possible data weighted by the probability that the real system produces such data.

\begin{equation}
E(h)=\int \ell(h(\vec{x},y) dP(\vec{x},y)
\end{equation}

\end{definition}

\begin{definition}[Empirical Error.]
\label{EmpiricalError}
The empirical error is the error calculated via a given loss function \(\ell\) over a subset \(D\) that represents the available data \(D \subset X \times Y\), where each sample is weighted equally. 

\begin{equation}
E_{d}(h)=\frac{1}{D}\sum_{(\vec{x},y)\in D}{\ell(h(\vec{x},y))}
\end{equation}

\end{definition}

In practice, the real system is unknown and the error has to be approximated using the available data \(D \subset X \times Y\). This approximation is called the \textbf{empirical error}. In some works, the definition of the empirical error is instead called \emph{risk}, denoted with \(R(h)\), and the term error is specifically used to refer to an error that is calculated with a binary loss function \citep{kouw2019}. The empirical error is related to the \emph{\ac{PAC}} learning framework because it can be used in empirical risk minimization. 

\subsubsection{Learning Frameworks}
\label{sec:appendix:concepts:ml:learning_frameworks}
Learning frameworks refer to how the definitions above are translated into the real world. They define under which conditions a hypothesis is selected and what restrictions are applied. In the scope of this work, two frameworks shall be briefly introduced, starting with \ac{PAC} learning. Here the goal is to select the best hypothesis \(h_s\) out of a set of possible hypotheses \(\mathcal{H}\). A formal definition is given by \citet{shalev-shwartz2014}. 

\begin{definition}[\ac{PAC} Learning.]
\label{PacLearning}
A hypothesis class \(\mathcal{H}\) is learnable if there exists an algorithm \(A\) which takes a sample \(S\) of size \(m\) that is sampled from probability distribution \(p\) and returns a predictor \(h_s=A(S) \in \mathcal{H} \)  for any given precision \(\epsilon > 0, \delta > 0\)  such that 

\begin{equation}
E(h_s)\leq \min_{h\in\mathcal{H}}E(h)
\end{equation}

with a confidence \(1-\delta\) provided that the sample \(m\) is large enough. 
\end{definition}

Given a complexity measure \(d[\mathcal{H}]\) of class \(\mathcal{H}\) that can e.g., be expressed as the VC-dimension \citep{vapnik1994} of the class, error bounds in \ac{PAC} typically look like 

\begin{equation}
\epsilon \leq a \cdot \sqrt{\frac{d[\mathcal{H}]+\log(1/\delta)}{m}}
\end{equation}

where \(a\) is a constant \citep{lemberger2020}. A different approach to \ac{PAC} is the \ac{MLA}. In \ac{MLA} a probability distribution \(\hat{P}(\vec{x},y)\) is learned to approximate the actual system \(P({x},y)\). This is a difference to \ac{PAC} that bypasses this step and immediately looks for a good predictor. According to \citet{meng1993}, \ac{MLA} can be defined as follows. 

\begin{definition}[\ac{MLA} Learning.]
\label{def:MlaLearning}
Given a probability distribution that is described by the parameters \(\theta\), select an approximation \(\theta_{ML}\) so that the log-probability of the observed samples \(S=\{(\vec{x}_1,y_1),...,(\vec{x}_m,y_m)\}\) is maximal. 

\begin{equation}
\theta_{ML}:=\text{arg max}_{\theta} \log(\prod_{i=1}^{m}{p_\theta(x_i,y_i))}
\end{equation}

\end{definition}

While PAC learning is usually more common in supervised approaches, some domain adaptation procedures that are presented in later chapters rely on maximum likelihood learning to perform the feature space alignment. 

\subsection{Transfer Learning and Domain Adaptation}
\label{sec:appendix:concepts:tl}

In the context of domain adaptation, there is no full consensus concerning definitions or terminology in the scientific community \citep{kouw2019a}. An important notion to understand is the difference between domain adaptation and transfer learning. The latter can be seen as the general case of utilizing knowledge between similar problems, which renders domain adaptation a special case of transfer learning. To make the differentiation more formal, more precise definitions are required. The vector notation used in \Ref{sec:appendix:concepts:ml} is omitted to improve the readability. 

\begin{definition}[Domain.]
\label{Domain}
A domain $D$ is described by a feature space $\mathcal{X}$ and a marginal probability distribution $P:X \rightarrow [0,1]$, where $X=\{x_1,...,x_n\} \in \mathcal{X}$.
$$D=\{\mathcal{X}, P(X)\}$$
\end{definition}

For example, in the popular MNIST data set, the original images of handwritten digits used by \citet{lecun1998} are 28x28 pixels in size, whereas each pixel is assigned a grayscale value of 0 (white) to 255 (black). If we consider the MNIST data set a domain, the feature space is $\mathcal{X}=\{0,...,255\}^{(28\cdot 28)}$ and the marginal probability distribution assigns each possible picture a probability according to the frequency of the picture in the data set. In reality, it is often non-trivial to determine the marginal probability distribution of a domain \citep{hoffman2018}.  

\begin{definition}[Task.]
\label{Task}
Given a specific domain $D$, a task $\mathcal{T}$ consists of a feature space $\mathcal{Y}$ and an objective predictive function $f(\cdot)$.
$$\mathcal{T}=\{\mathcal{Y}, f\}$$ 
\end{definition}

Often the objective predictive function is based on the conditional probability function $f(x_j)=\{P(y_k|x_j) | y_k \in \mathcal{Y}, k=1,...,|\mathcal{Y}|\}$, which can be learned in a supervised manner from the labeled data $\{x_i,y_i\} \in X \times Y $. For example, in a classification  problem, we are observing the features $x_i \in X$ and deciding for a class $y_i \in Y$. In the example of the MNIST data set, each picture is a handwritten digit, i.e., $\mathcal{Y}=\{0,1,...,9\}$. In some instances, the objective predictive function is not defined as a marginal probability of an output $Y$ given observed data $X$, but instead directly assigns the output $f':X \rightarrow Y$ by some rule, e.g., maximum probability. For simplicity, in the next definitions, we assume that the conditional probability is the only relevant parameter for the objective prediction function, i.e., $f_{P(Y|X)}: X \rightarrow Y$, and adapt the task definition to reflect that: $\mathcal{T}=\{\mathcal{Y}, P(Y|X)\}$. 

Given two domains, a source domain $D^s$ and target domain $D^t$, with tasks $\mathcal{T}^s$ and $\mathcal{T}^t$, traditional \ac{ML} has the same domains for training and test data sets, $D^s=D^t$, and the same tasks $\mathcal{T}^s=\mathcal{T}^t$. A divergence can be caused by either a domain divergence, a task divergence, or both. 

\begin{definition}[Domain Divergence.]
\label{DomainDivergence}
Given two domains $D^s=\{\mathcal{X}^s, P^s(X^s)\}$ and $D^t=\{\mathcal{X}^t, P^t(X^t)\}$, a discrepancy between two domains can be caused by either a difference in the distribution $P^s(X^s) \neq P^t(X^t)$, called \textbf{distribution shift} or \textbf{covariate shift}, in the feature space $\mathcal{X}^s \neq \mathcal{X}^t$, called \textbf{feature space difference}, or both.
\end{definition}

\begin{definition}[Task Divergence.]
\label{TaskDivergence}
Given two  tasks\\ $\mathcal{T}^s=\{\mathcal{Y}^s, P^s(Y^s|X^s)\}$ and $\mathcal{T}^t=\{\mathcal{Y}^t, P^t(Y^t|X^t)\}$, a discrepancy between two tasks $\mathcal{T}^s, \mathcal{T}^t$ can be either due to a \textbf{conditional distribution shift} $P^s(Y^s|X^s) \neq P^t(Y^t|X^t)$, a \textbf{label space difference} $\mathcal{Y}^s \neq \mathcal{Y}^t $, or both.
\end{definition}

Transfer learning is defined as the learning scenario where a model is trained on a source domain or task and evaluated on a different but related domain or task, where either the tasks or domains, or both, differ \citep{wilson2020}. A precise definition that includes the multi-domain case is given by \citet{zhuang2020}.

\begin{definition}[Transfer Learning.]
\label{TransferLearning}
Given some/an observation(s) corresponding to $m^S\in \mathbb{N}^+$ source domain(s) and task(s), and some/an observation(s) about $m^T \in \mathbb{N}^+$ target domain(s) and task(s), transfer learning utilizes the knowledge implied in the source domain(s) to improve the performance of the learned decision functions $f^{T_j} (j=1,...,m^T)$ on the target domains. 
\end{definition}

Utilizing the formal definitions of possible divergences for a \ac{ML} problem, the differentiation of domain adaptation from transfer learning can be made by defining a subset of transfer learning problems that adhere to the following restrictions.

\begin{definition}[Domain Adaptation.]
\label{DomainAdaptation}
Domain adaptation considers all transfer learning solutions with the assumption that the task(s) between domains remain(s) the same $\mathcal{T}^s = \mathcal{T}^t$, and the differences are only caused by domain divergence, i.e., $D^s \neq D^t$  \textnormal{\citep{wang2018}}. 
\end{definition}

Domain adaptation problems can be further classified by incorporating the reason for the domain divergence, or the availability of labeled data in the target domain. A domain adaptation problem is called \emph{homogeneous} if the feature space remains the same between the source and the target domain, i.e., $\mathcal{X}^s = \mathcal{X}^t$ and the reason for the difference is only due to different probability distributions. A domain adaptation problem is called \emph{heterogeneous} if it is not homogeneous, i.e., if the feature spaces are not equal between the source and target domain. 

In most domain adaptation problems,  it is generally assumed that labels are available for all source data points. As this is not the case for the target domain, we can further classify problems based on the availability of target labels \citep{wang2018}. Assuming a completely labeled source domain $D^s=\{\mathcal{X}^s, P(X)^s\} $ and a target domain with a small amount of labeled data or no labeled data $D^t=\{\mathcal{X}^t, P(X)^t\} $, we can split up the target domain into a labeled part $D^{tl}$ and an unlabeled part $D^{tu}$, which together form the entire target domain $D^t = D^{tl} \cup D^{ul} $. In the source domain, a task $\mathcal{T}^s$ can be learned from labeled data points $\{x_i^s,y_i^s\}$. In the target domain, a task $\mathcal{T}^t$ can be learned from both labeled data $\{x_i^{tl},y_i^{tl}\}$ and unlabeled data $\{x_i^{tu}\}$. A domain adaptation problem is called \emph{supervised}, if all target data is labeled $D^t = D^{tl}$. Domain adaptation can still be required because the overall amount of labeled target data might be too small to sufficiently train a model. A domain adaptation problem is called \emph{semi-supervised}, if both labeled and unlabeled target data is present $D^t = D^{tl} \cup D^{ul} $. Commonly, only a small amount of target data is labeled, which motivates the use of domain adaptation methods. A domain adaptation problem is called \emph{unsupervised}, if all target data is unlabeled $D^t = D^{tu}$. 

\subsection{Divergence Measures}
\label{sec:appendix:concepts:divergence_measures}
It is often difficult to express the difference between domains (or tasks) in quantitative terms. If the feature (or label) space remains constant, the difference of a domain (or task) can be expressed by the difference in the distribution $P(x)$ (or $P(y|x)$) between the source and target domain. Measuring the difference between two probability distributions is an ongoing topic in statistics and information theory. Many domain adaptation implementations rely on some form of divergence measure for probability distributions.

The \emph{Kullback-Leibler divergence} $D_{KL}$ was proposed by \citet{kullback1951} and measures the difference between two probability distributions. It is also known as the relative entropy. In information theory, the Kullback-Leibler divergence states how many additional bits are needed on average to encode a message using a code optimized for probability distribution Q if the message actually is from a source with probability distribution P. 

\begin{definition}[Kullback-Leibler Divergence.]
\label{def:KullbackLeibler}
For discrete probability distributions $P$ and $Q$ defined on the same probability space $\mathcal{X}$, the Kullback-Leibler divergence $D_{KL}$ from $Q$ to $P$ is  
\begin{equation}
 D_{KL}(P||Q)=\sum_{x\in \mathcal{X}}P(x) \log \left(\frac{P(x)}{Q(x)} \right) \in [0, \infty).
\end{equation}
For distributions $P$ and $Q$ of two continuous random variables, the sum is replaced by an integral
\begin{equation}
D_{KL}(P||Q)=\int_{x\in \mathcal{X}}P(x) \log \left(\frac{P(x)}{Q(x)}\right)dx \in [0, \infty).
\end{equation}
\end{definition}

It is apparent that the Kullback-Leibler divergence is not symmetric, i.e., $D_{KL}(P||Q) \neq D_{KL}(Q||P)$, and therefore not a metric. The lower bound of the Kullback-Leibler divergence is 0, which is achieved if the probability distributions are identical. There is no upper bound, which can be an undesired property.

The \emph{Jensen-Shannon divergence} $D_{JS}$ is another measure for the similarity of two probability distributions that aims to mitigate these weaknesses by using a symmetrized and smoothed version of the Kullback-Leibler divergence \citep{fuglede2004}. If the base 2 logarithm is used, the Jensen-Shannon divergence is bounded as $0 \leq D_{JS}(P||Q) \leq 1$. The square root of the Jensen-Shannon divergence fulfills the requirements for a metric and is sometimes referred to as the Jensen-Shannon metric. 

\begin{definition}[Jensen-Shannon Divergence.]
\label{def:Jensen-Shannon}
For probability distributions $P$ and $Q$ of two continuous random variables from the same probability space $\mathcal{X}$, the Jensen-Shannon divergence $D_{JS}$ is defined as
\begin{equation}
    D_{JS}(P||Q)=\int_{x\in \mathcal{X}}P(x)\log \left (\frac{P(x)}{\frac{1}{2}P(x)+\frac{1}{2}Q(x)} \right ) dx. 
\end{equation}
\end{definition}

Another related similarity measure that is sometimes used is called the \emph{R\'{e}nyi divergence} $D_{\alpha R}$ \citep{vanerven2014}. It introduces a parameter $\alpha$ that is referred to as the order of the divergence. For $\alpha=1$ the R\'{e}nyi divergence is the Kullback-Leibler divergence.

\begin{definition}[R\'{e}nyi Divergence.]
\label{def:RenyiDivergence}
For probability distributions $P$ and $Q$ of two continuous random variables from the same probability space $\mathcal{X}$, the R\'{e}nyi divergence $D_{\alpha R}$ is 
\begin{equation}
D_{\alpha R}(P||Q)=\frac{1}{\alpha -1}\log_2 \int_{x \in \mathcal{X}}P^\alpha(x)\/Q^{\alpha -1}(x) dx, 
\end{equation}
where $\alpha$ denotes the order of the divergence.
\end{definition}

The difference between two probability distributions may also be expressed via a concept that is not related to some definition of entropy. An example of this is the \emph{\ac{MMD}} that represents the difference of distributions as the distance between mean embeddings of the features \citep{borgwardt2006} via a kernel. For many kernels, including the Gaussian kernel, the \ac{MMD} is only zero if the compared distributions are identical. The \ac{MMD} can be estimated from a sample using the kernel trick to avoid calculations in the kernel space. 

\begin{definition}[Maximum Mean Divergence.]
\label{def:MaximumMeanDivergence}
Given two probability distributions $P$ and $Q$, the \acl{MMD} MMD is given by 
\begin{equation}
    \text{MMD}(P,Q)=||\mathbb{E}_{X\sim P}[\varphi (X)] - E_{Y \sim Q}[\varphi (Y)]||_{\mathcal{H}},
\end{equation}
whereas $\varphi : \mathcal{X} \to \mathcal{H} $ is a feature map that maps to a reproducing kernel Hilbert space $\mathcal{H}$. 
\end{definition}

% There are also divergence measures that are not as relevant from a practical point of view, but instead used in theoretical statements. An example for this is the \emph{symmetric difference hypothesis divergence} $D_{\mathcal{H}\Delta \mathcal{H}}$ that compares two distributions based on the largest disagreements of two classifiers $h,h' \in \mathcal{H}$ from a set of classifiers $\mathcal{H}$ \citep{ben-david2010}. 

% \begin{definition}[Symmetric Difference Hypothesis Divergence]
% \label{def:SymmetricDifferenceHypothesisDivergence}
% For two probability distributions $P$ and $Q$, the symmetric difference hypothesis divergence $D_{\mathcal{H}\Delta \mathcal{H}}$ over a set of hypothesis $\mathcal{H}$ is defined as 
% \begin{equation}
% \begin{split}
%     D_{\mathcal{H}\Delta \mathcal{H}}(P,Q) = \\
%     2 \sup_{h,h'\in \mathcal{H}} |Pr_P[h(x)\neq h'(x)|]-Pr_Q[h(x) \neq h'(x)]|.
% \end{split}
% \end{equation}
% \end{definition}

\section{Transformation Function in Class-conditional Shift}
\label{sec:appendix:ClassConditionalShift}

\begin{prop}
\label{prop:ClassConditionalShift}
If there exists a transformation function $t$, so that $P_s(x|y) = P_t\left(t\left(x\right)|y\right), \forall y\in Y$, then this transformation function can be also observed in the feature space $P_s(x)=P_t(t(x))$ assuming a class-conditional shift and pairwise disjoint classes.
\end{prop}

\begin{proof}
From the law of total probability \cite{pfeiffer1978}, it holds that  
\begin{equation}
\label{eq:TotalProbability}
    P_i(x)=\sum_{y \in Y} P_i(x|y) \cdot P_i(y), \quad x \in X
\end{equation}
for domains $i \in \{s,t\}$ and pairwise disjoint classes. Now let $t\colon X \to X$ be the transformation such that 
\begin{equation}
\label{eq:transformation}
    P_s(x|y)=P_t\left(t\left(x\right)|y\right), \quad \forall x \in X, y\in Y.    
\end{equation} 
Using Equation \ref{eq:transformation} and the equality of priors in a class-conditional shift, i.e. $P_s(y)=P_t(y), y \in Y$, we get
\begin{equation}
\begin{split}
    P_t(t(x)) &= \sum_{y \in Y} P_t\left(t\left(x\right)|y\right) \cdot P_t(y) \\
    &= \sum_{y \in Y} P_s(x|y) \cdot P_s(y) \\
    &= P_s(x)
\end{split}
\end{equation}
\noindent
for all $x \in X$.
\end{proof}
